# Supplementary material for: GeoSAM2: Unleashing the Power of SAM2 for 3D Part Segmentation
Source: arXiv:2508.14036 source file (2025-08-27)

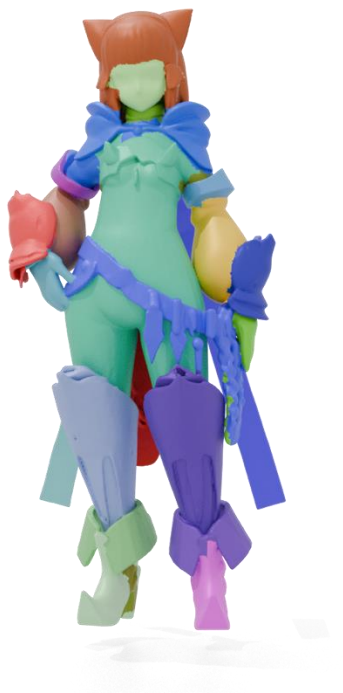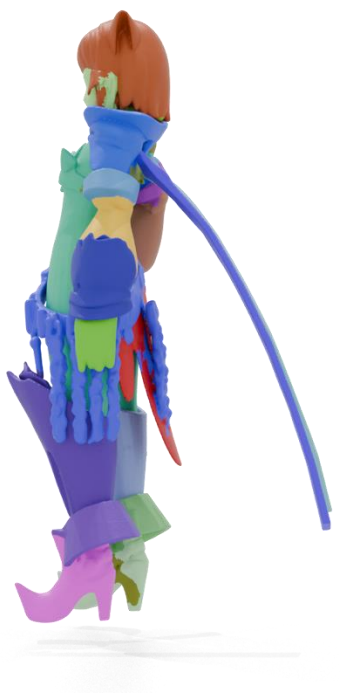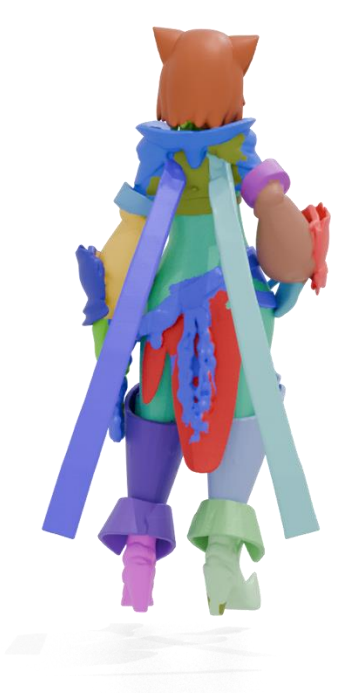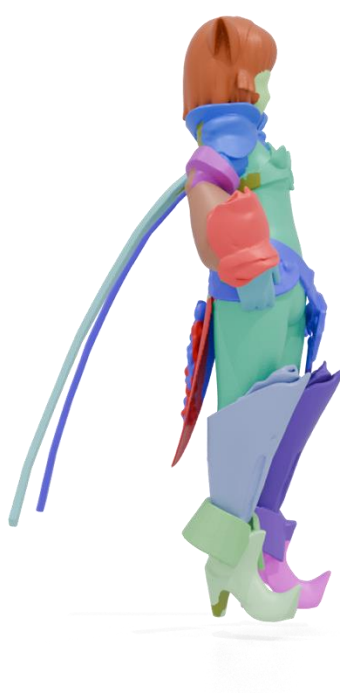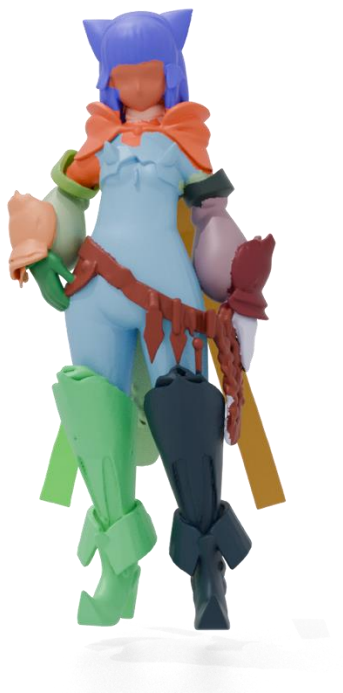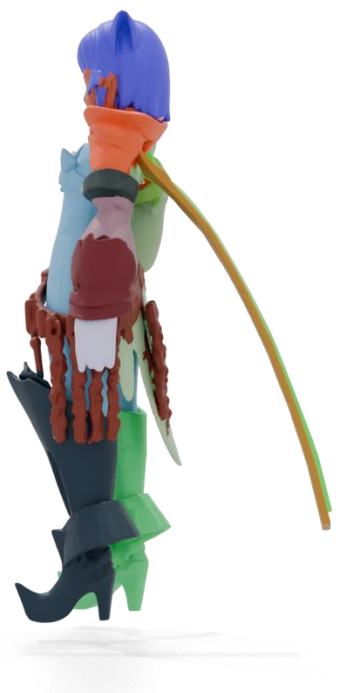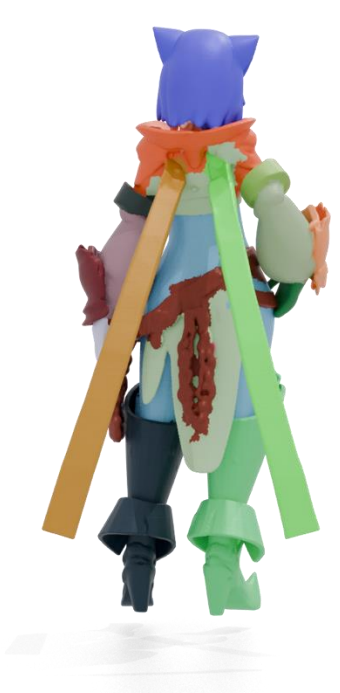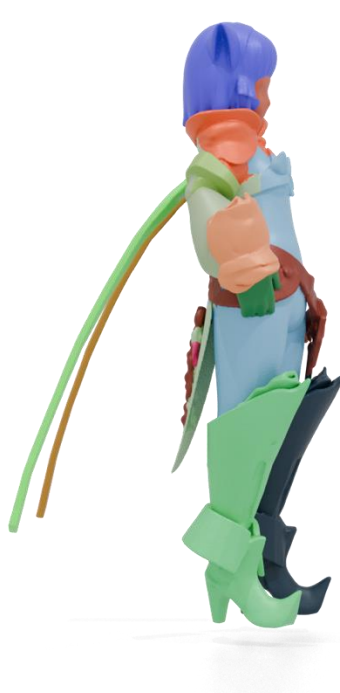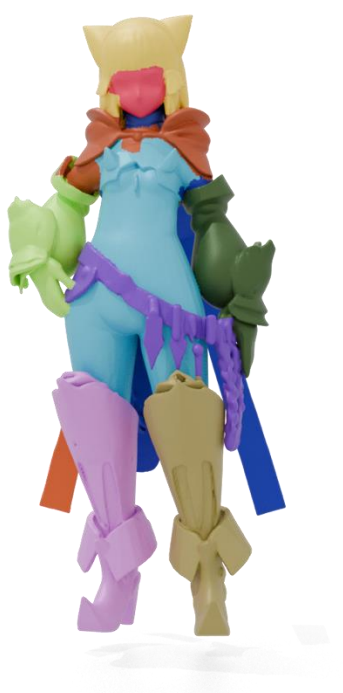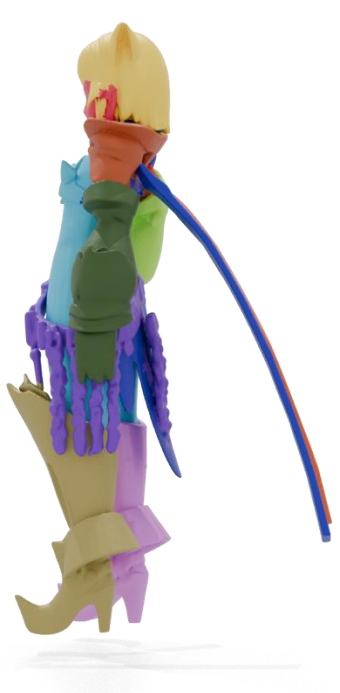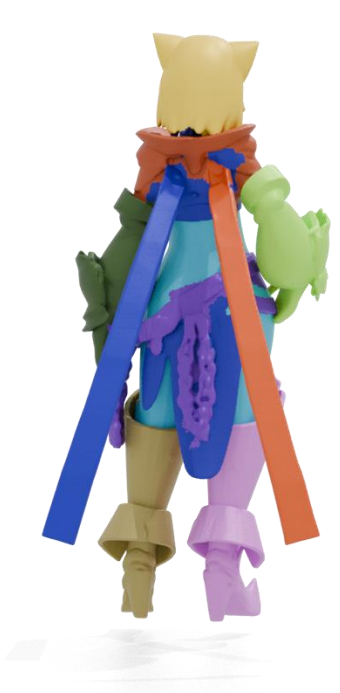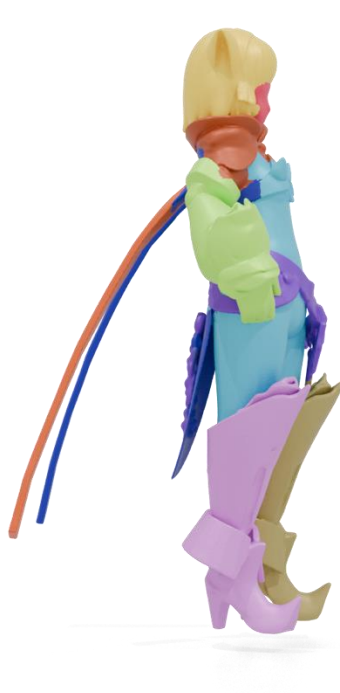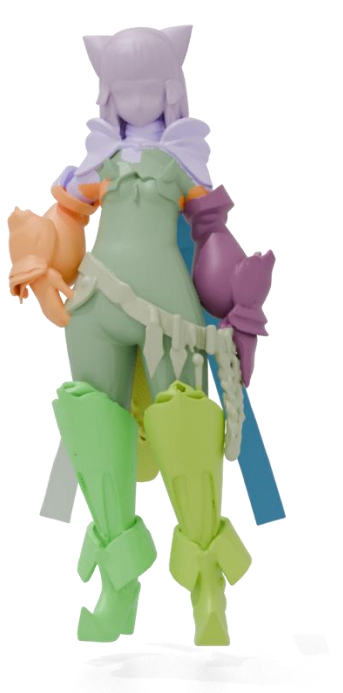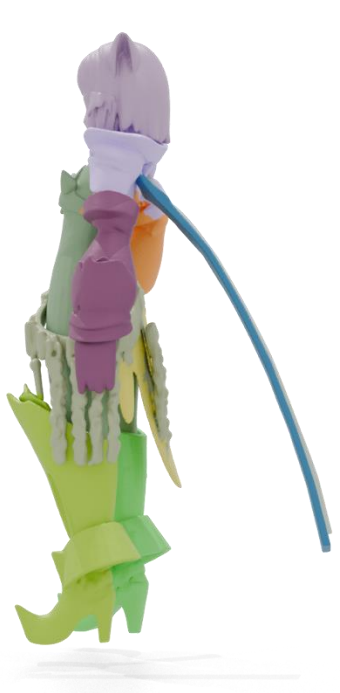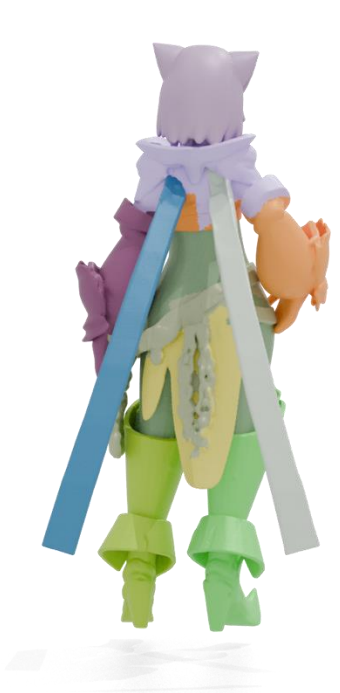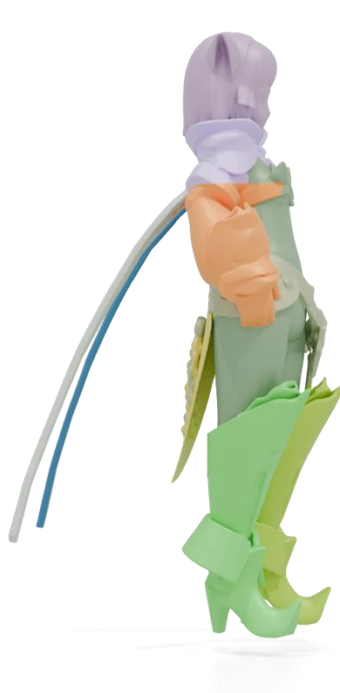

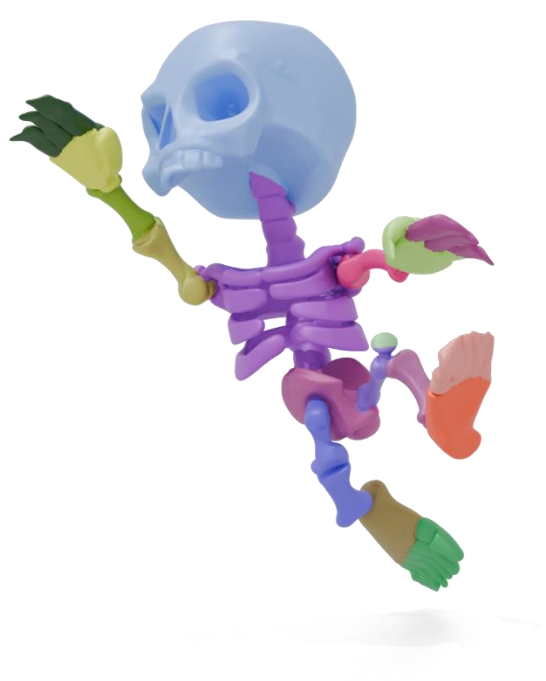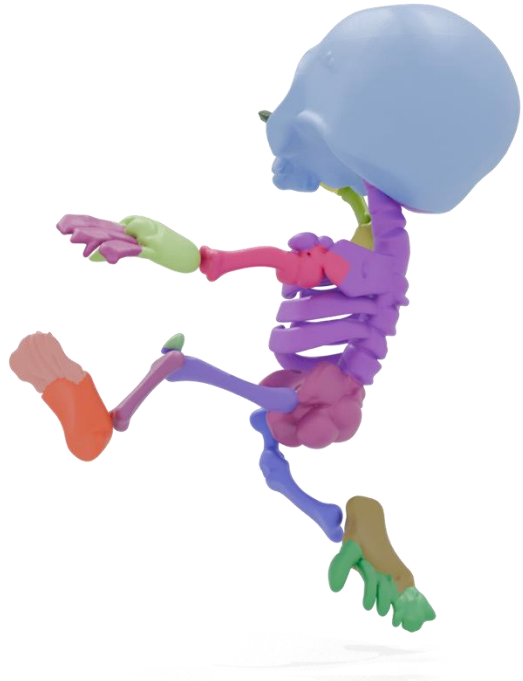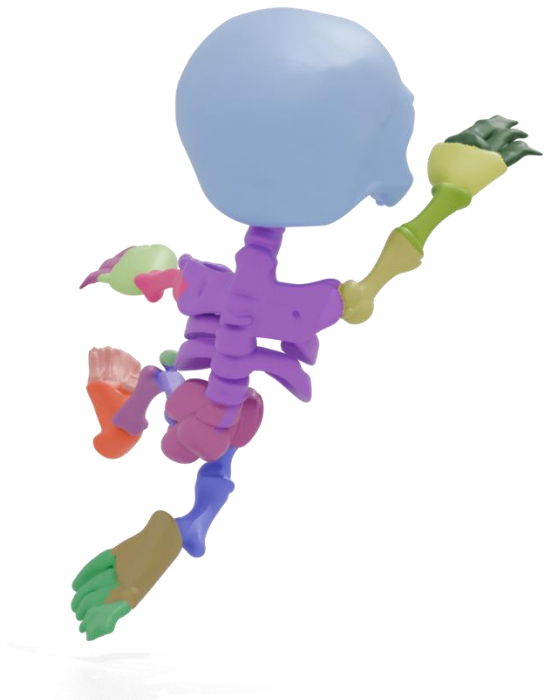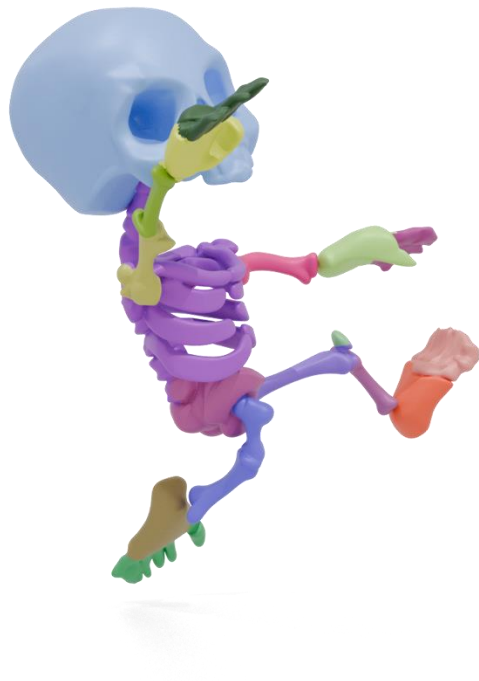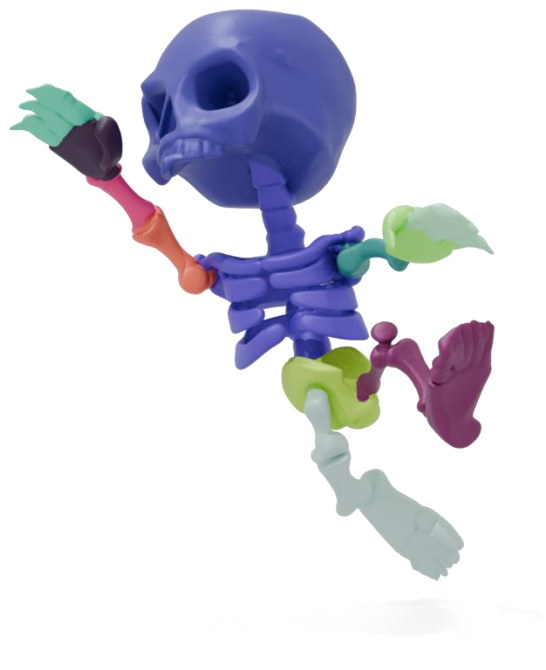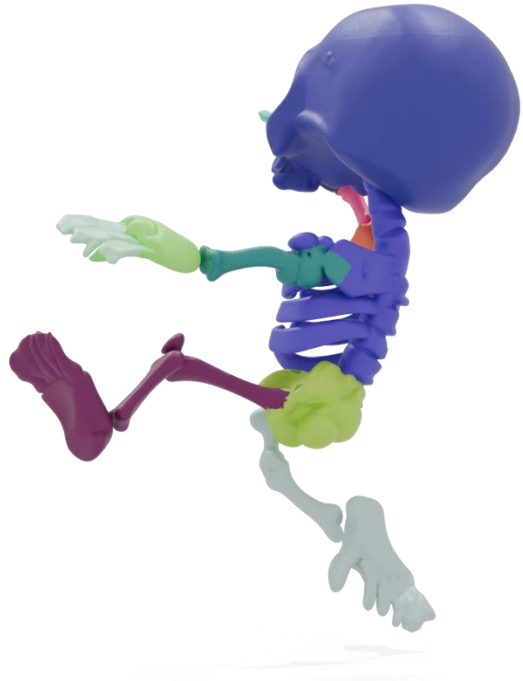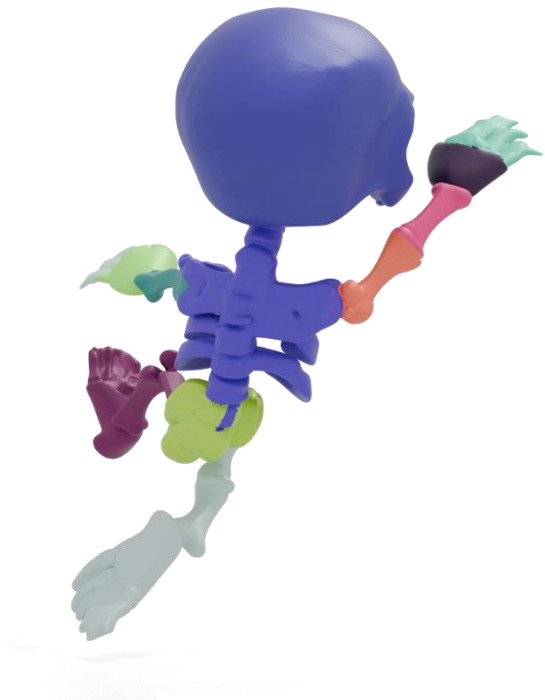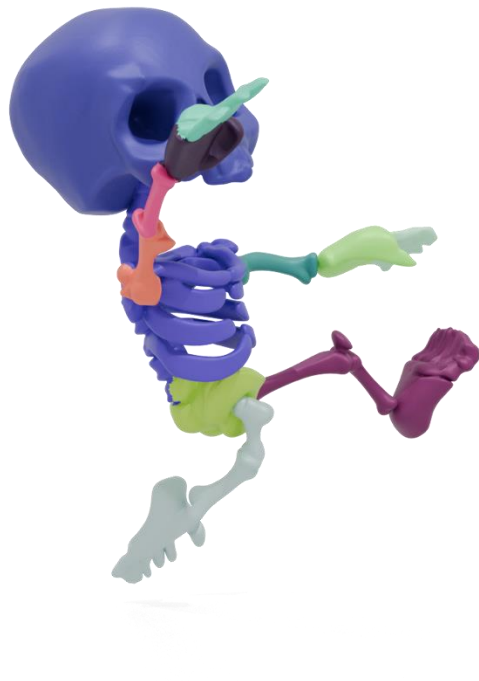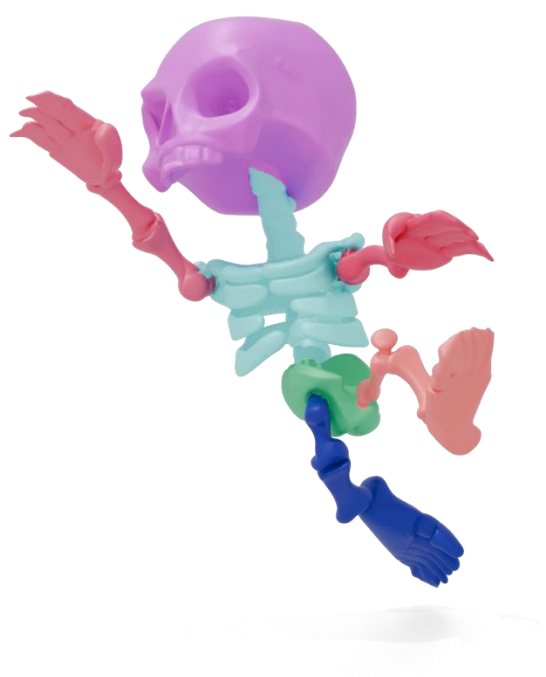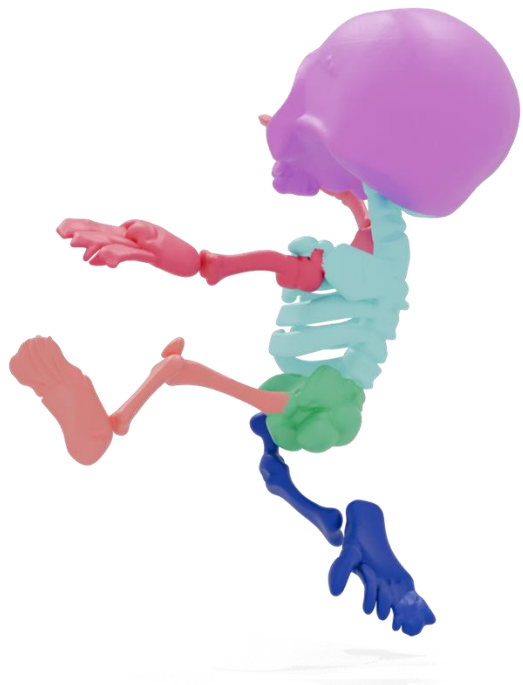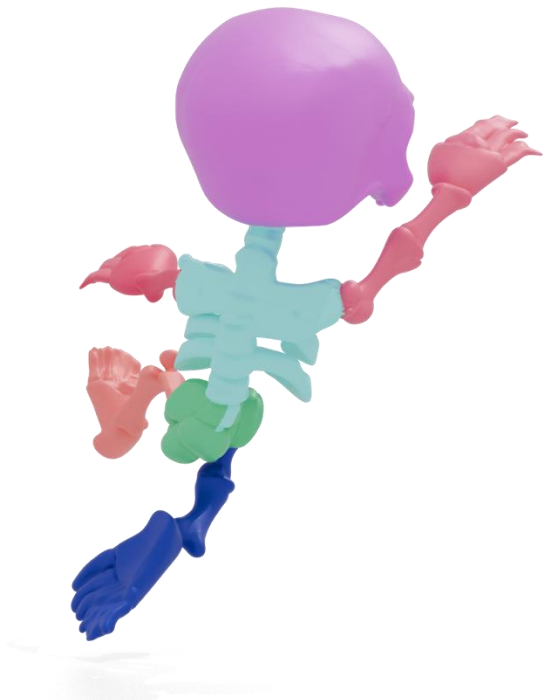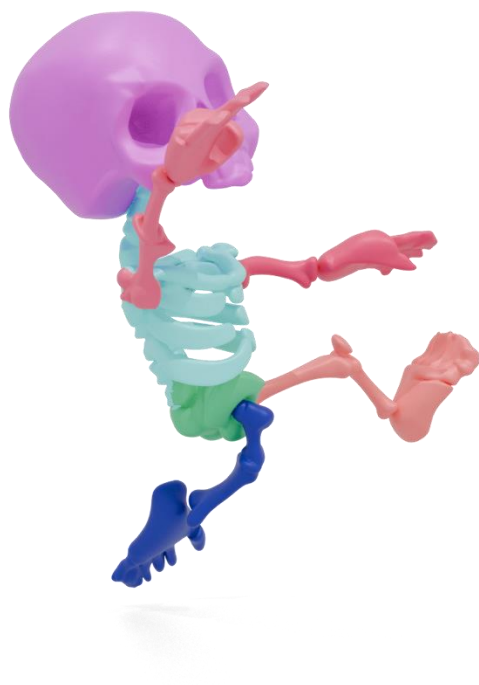



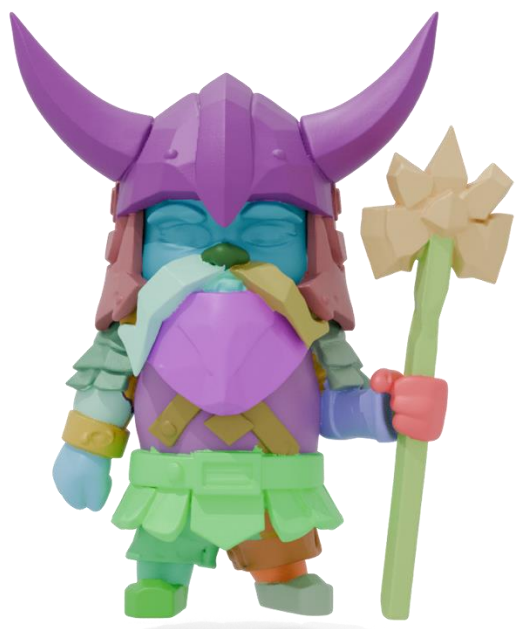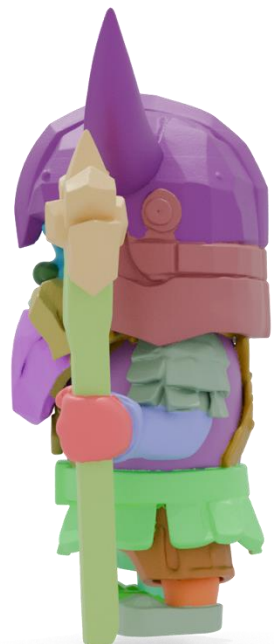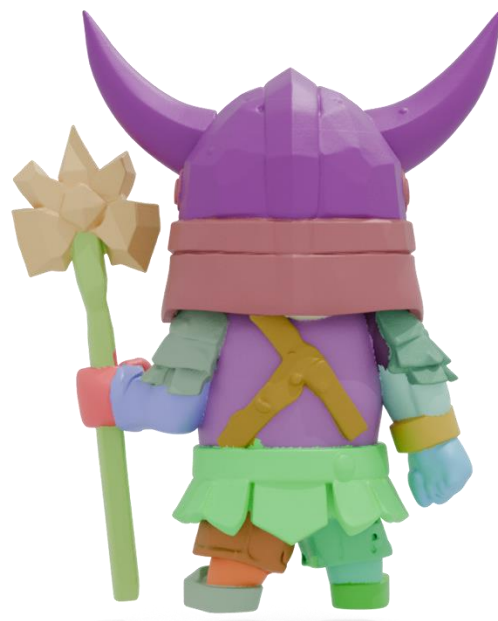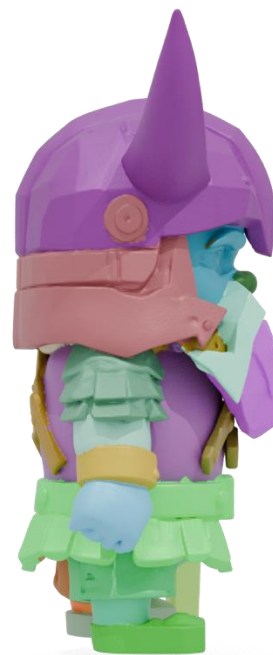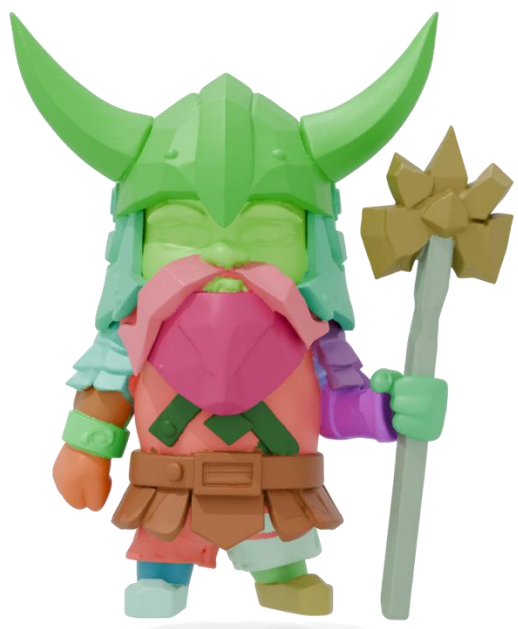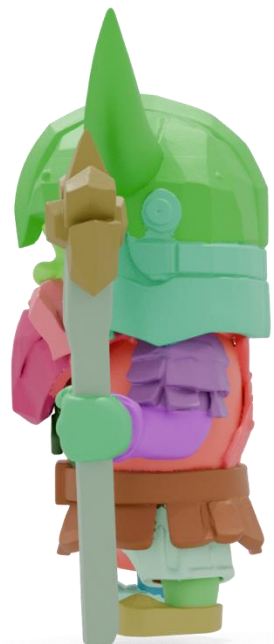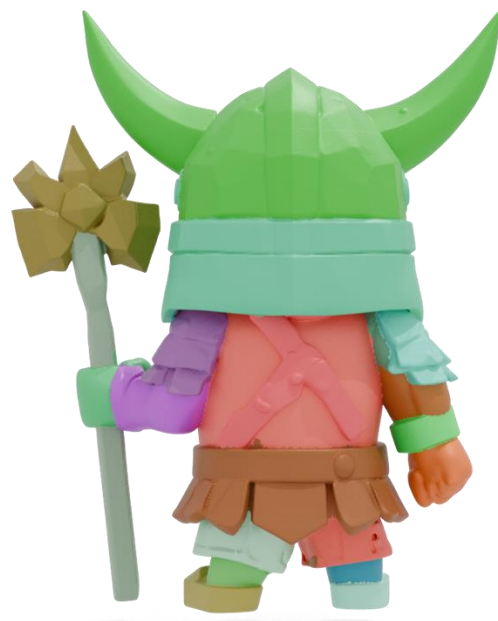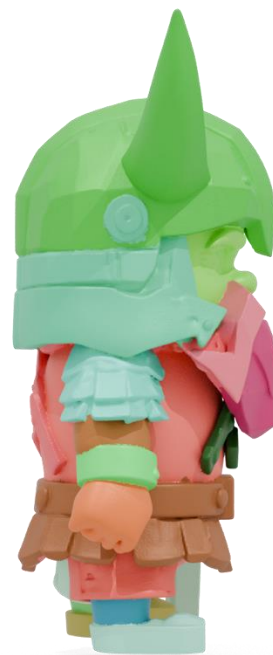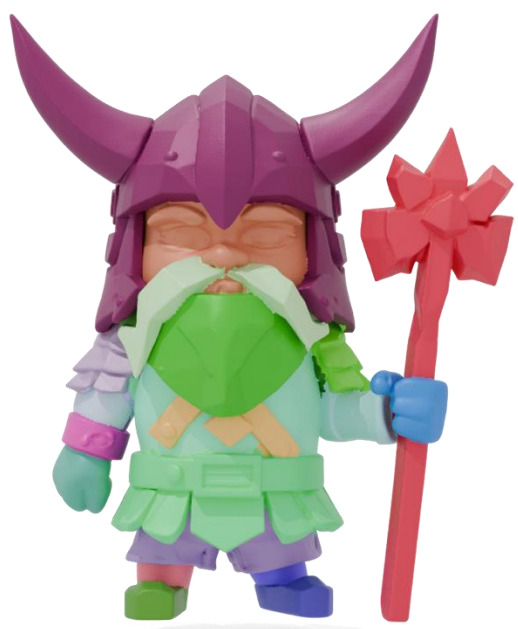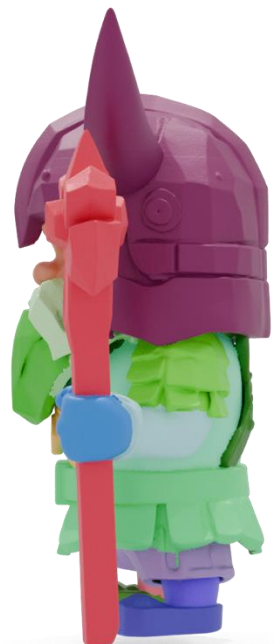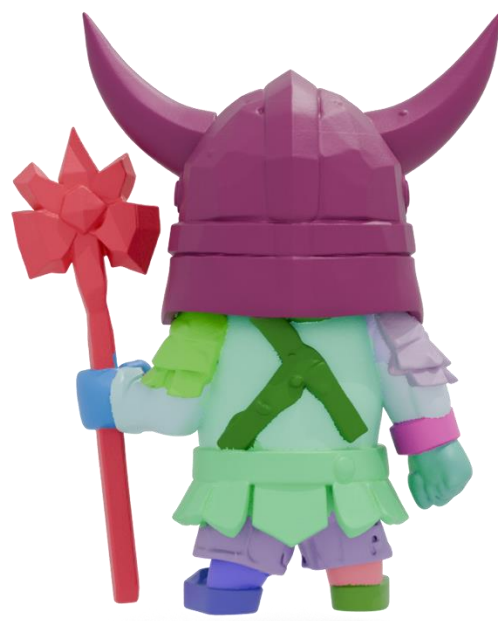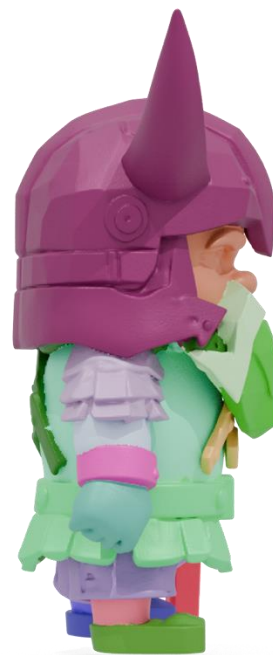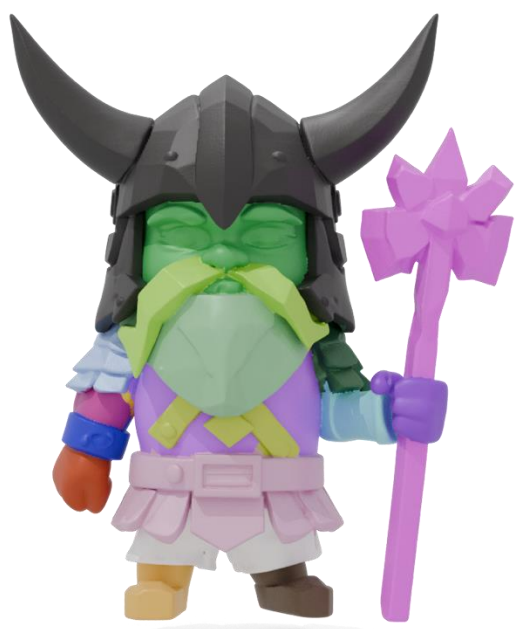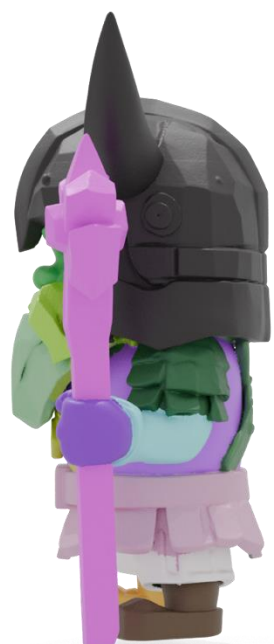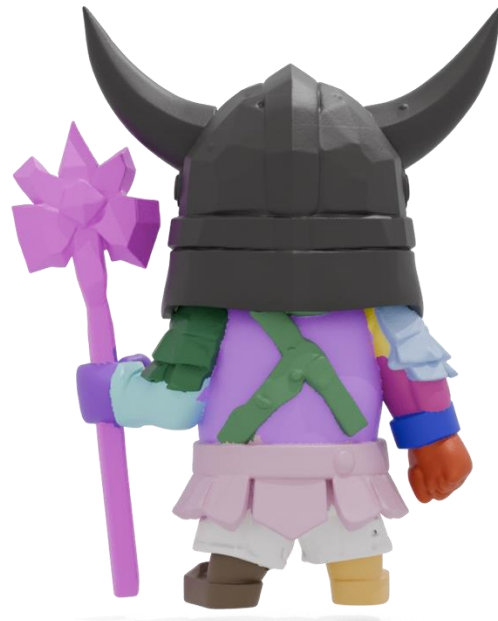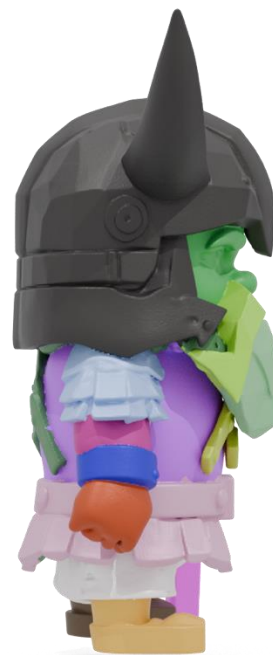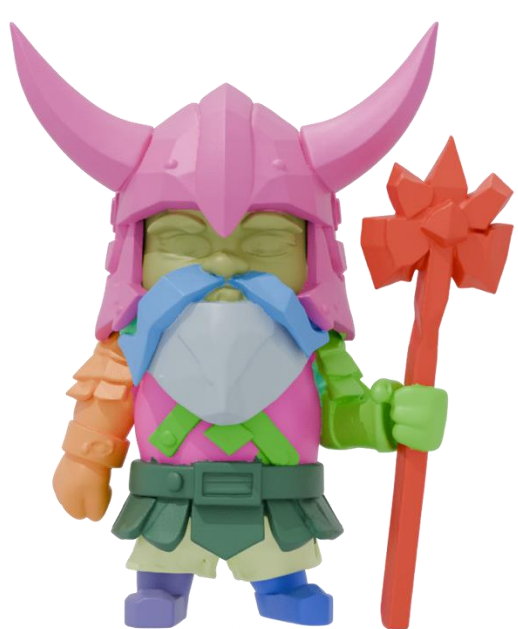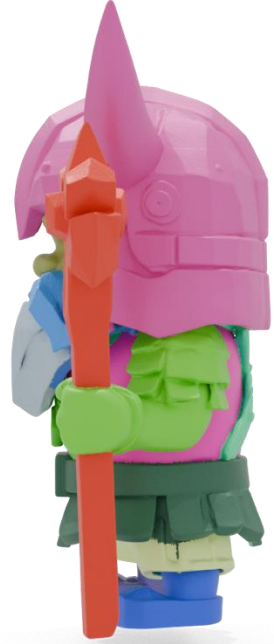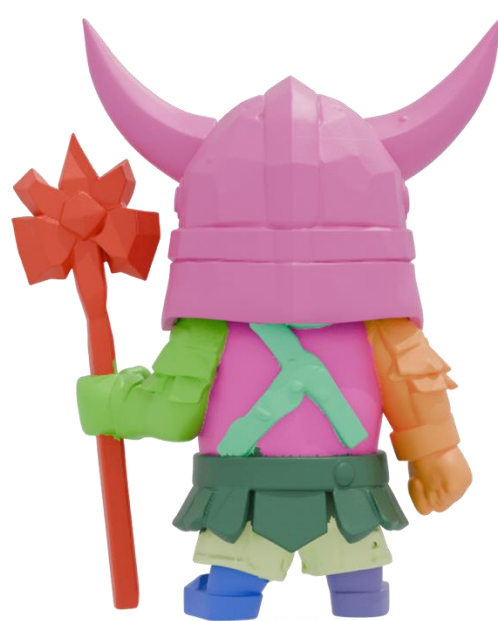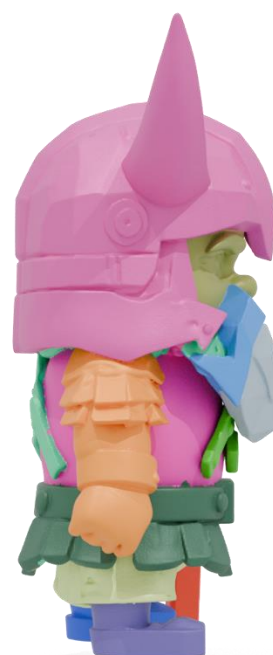

Supplement: Supplementary file 1 [file supp_hierarchy.pdf]
